# Supplementary material for: Implicit energy regularization of neural ordinary-differential-equation control
Source: arXiv:2103.06525 ancillary file (2021-03-11)
Supplement: Supplementary file 1 [file OPTIMAL_CONTROL_SI.pdf]

# Supplemental Information: Implicit energy regularization of neural ordinary-differential-equation control

Lucas Böttcher,[1,*] Nino Antulov-Fantulin,[2,†] and Thomas Asikis[2,‡]

[1] *Computational Medicine, University of California, Los Angeles, 90095-1766, Los Angeles, United States*

[2] *Computational Social Science, ETH Zurich, 8092, Zurich, Switzerland*

(Dated: March 11, 2021)

## I. CONTROL OF KURAMOTO DYNAMICS

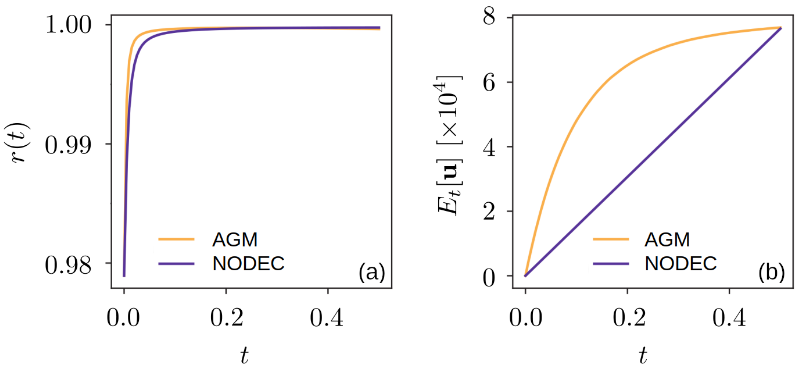


FIG. 1. Control of Kuramoto dynamics on a square lattice with $50 \times 50$ nodes. NODEC and the AGM reach a similar (a) order parameter and (b) control energy at $T = 0.5$. As in the main text, we set $K = 0.1K^*$.

Here we demonstrate the ability of NODEC to control larger systems than than those used in the main text. As an example, we consider Kuramoto dynamics [Eqs. (11) and (12) in the main text] on a square lattice with $50 \times 50$ nodes (Fig. 2). The control horizon is $[0, T]$ with $T = 0.5$. We compare the control performance of NODEC with that of the adjoint-gradient method [AGM, Eqs. (18) and (19) in the main text]. Figures 2(a) and (b) show the corresponding evolution of the order parameter and control energy, respectively. Both NODEC and the AGM reach similar order parameter and control energy values at time $T = 0.5$, indicating that the control performance of both methods is similar. This result is further supported by the data in Fig. 2, showing that the Kuramoto system is synchronized around $\theta_i(T) = 0$ by both algorithms in a similar manner.

| Controller | Runtime per Loop | Total Loops | Total Runs |
|---|---|---|---|
| AGM | $74$ s $\pm\ 25.6$ ms | 10 | 5 |
| NODEC | $1.03$ s $\pm\ 511$ $\mu$s | | |

TABLE I. Training time performance of NODEC and the AGM. Each controller is retrained for each loop. We perform 10 loops per run and 5 runs in total and select and report the mean runtime per loop and the corresponding standard deviation of the run with the lowest mean runtime.

* lucasb@ucla.edu
† anino@ethz.ch
‡ asikist@ethz.ch

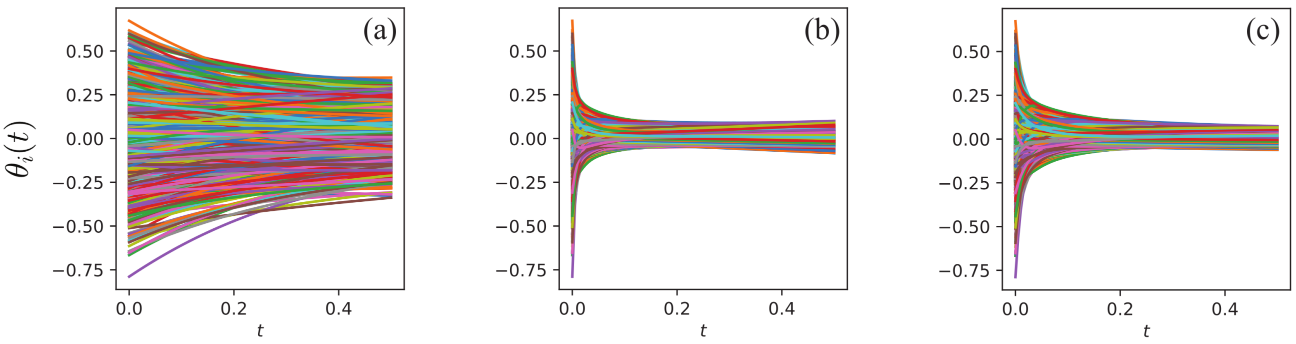


FIG. 2. Kuramoto dynamics on a square lattice with $50 \times 50$ nodes. The plots show the evolution of the phase angles $\theta_i(t)$ of all nodes for (a) no control, (b) AGM-controlled dynamics, and (c) NODEC-controlled dynamics.

For a runtime performance comparison, we also measured the real-world learning time (or wall-clock time) using the command `timeit` in `python`. We find that the training time of NODEC is about two orders of magnitude smaller than that of the AGM (Table I). Both algorithms, NODEC and the AGM, are implemented in `pytorch`.

## II. NEURAL-NETWORK ARCHITECTURES AND HYPERPARAMETERS

All neural networks that we use to represent the control input $\hat{\boldsymbol{u}}(t;\boldsymbol{w})$ take the time $t$ as an input. To numerically integrate the studied dynamical systems, we apply the Dormand–Prince (DOPRI) method during training and evaluation [1].

In the following paragraphs, we summarize the neural-network architectures and hyperparameters that we used in our numerical experiments.

*Two-state system.* The neural network consists of a single hidden layer with 6 neurons and an exponential linear unit (ELU) activation. We transform the hidden layer output to the control signal via a linear layer with 1 neuron that describes the single control input in Eq. (8) (main text). We initialize the neural-network weights $\boldsymbol{w}$ with the Kaiming uniform initialization algorithm [2]. For the gradient descent in $\boldsymbol{w}$ [Eq. (4), main text], we use a learning rate $\eta = 0.02$.

*Kuramoto model.* The neural-network hyperparameters for controlling Kuramoto dynamics are summarized in Table II. Independent of the underlying graph, we use the same number of hidden layers, hidden layer neurons, and training epochs. The activation function is (ELU) is also the same in all numerical experiments.

| Graph | Learning Rate | # Hidden Layers | # Hidden Layer Neurons | Activation | Training Epochs |
|---|---|---|---|---|---|
| Complete | 0.4 | 1 | 2 | ELU | 2 |
| Erdős–Rényi | 0.4 | | | | |
| Square lattice ($15 \times 15$) | 0.32 | | | | |
| Watts-Strogatz | 0.31 | | | | |
| Square lattice ($50 \times 50$) | 0.0125 | | | | |

TABLE II. Neural-network hyperparameters used for learning the control of Kuramoto dynamics on different graphs. All neural networks use stochastic gradient descent for learning and only differ in their learning rate. We include a bias term at each node and set all weights initially to a value of 0.001.

[1] J. R. Dormand and P. J. Prince, Journal of Computational and Applied Mathematics **6**, 19 (1980).
[2] K. He, X. Zhang, S. Ren, and J. Sun, in *Proc. IEEE Int. Conf. Comput. Vis.* (2015) pp. 1026–1034.
